# Supplementary material for: C2FAR: Coarse-to-Fine Autoregressive Networks for Precise Probabilistic Forecasting
Source: arXiv:2312.15002 source file (2023-12-22)
Supplement: Supplementary file 1 [file cross_dataset.tex]

\begin{table}
\caption{Summary of results across datasets\label{tab:cross_dataset}}
\footnotesize
\begin{tabular}{@{}llll@{}}
\toprule
                        & Num. 1st   & Num. 2nd   & Num. 3rd
\\ \midrule
\textbf{$\ctofarone$}   & \textbf{0} & \textbf{1} & \textbf{3} \\
\textbf{$\ctofartwo$}   & \textbf{1} & \textbf{3} & \textbf{0} \\
\textbf{$\ctofarthree$} & \textbf{3} & \textbf{0} & \textbf{1}
\\ \bottomrule
\end{tabular}
\end{table}
